# Supplementary material for: AutoDiscovery: Open-ended Scientific Discovery via Bayesian Surprise
Source: arXiv:2507.00310 source file (2026-02-12)
Supplement: Supplementary file 1 [file _supplementary.tex]

\documentclass{article}

\usepackage{neurips_2025}

\usepackage[utf8]{inputenc} %
\usepackage[T1]{fontenc}    %
\usepackage{hyperref}       %
\usepackage{url}            %
\usepackage{booktabs}       %
\usepackage{amsfonts}       %
\usepackage{nicefrac}       %
\usepackage{xcolor}         %

\usepackage{enumitem}
\usepackage{graphicx}
\usepackage{subcaption}
\usepackage{wrapfig}
\usepackage{algorithm}
\usepackage{algpseudocode}
\usepackage{amsmath}
\usepackage{bbm}
\usepackage{minted}
\usepackage{rotating}
\usepackage{tikz}

\algrenewcommand{\algorithmiccomment}[1]%
  {\Statex\hskip\algorithmicindent {\color{gray}$\triangleright$~#1}}

\input{macros}
\input{utils}

\title{\emph{Supplementary for} \\Open-ended Scientific Discovery via Bayesian Surprise}

\author{%
  David S.~Hippocampus\thanks{Use footnote for providing further information
    about author (webpage, alternative address)---\emph{not} for acknowledging
    funding agencies.} \\
  Department of Computer Science\\
  Cranberry-Lemon University\\
  Pittsburgh, PA 15213 \\
  \texttt{hippo@cs.cranberry-lemon.edu} \\
}

\begin{document}

\maketitle

\tableofcontents
\newpage

\section{Project Code}
We have anonymized and included the code used to run all experiments in this project as $\texttt{project\_code.zip}$ within the uploaded supplementary zip file.

\input{sections/supplementary/discovery_agent}
\input{sections/supplementary/algorithms}
\input{sections/supplementary/annotations}
\input{sections/supplementary/deduplication_analysis}
\input{sections/supplementary/o4_mini}
\input{sections/supplementary/examples_errors}

\end{document}
